# Supplementary material for: Vision-Language Pre-Training for Multimodal Aspect-Based Sentiment Analysis
Source: arXiv:2204.07955 source file (2022-04-21)
Supplement: Supplementary file 1 [file Appendix.tex]

\clearpage
\appendix
\section{Appendix}

% \captionsetup[table]{width=1\textwidth}
\begin{table}[H]
  \setlength{\belowcaptionskip}{-0.5cm}
  \setlength{\abovecaptionskip}{0.1cm}
  \scriptsize
\begin{tabular}{p{0.8cm}p{3.2cm}p{3cm}p{3.5cm}p{3.2cm}}
\toprule
Image &
\begin{minipage}{0.1\textwidth}
    \hbox{\hspace{-0.3em} \includegraphics[width=32mm, height=25.0mm]{./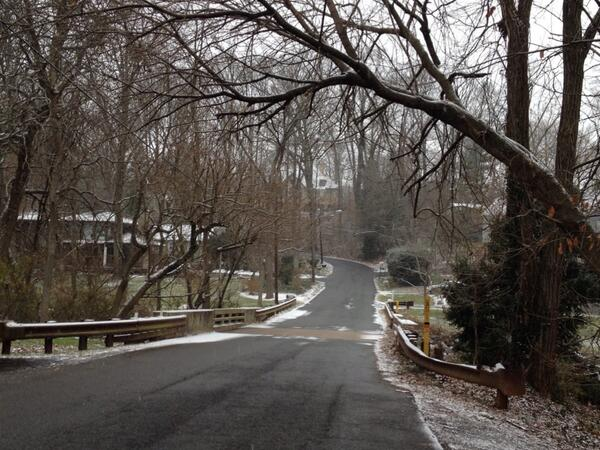}}
  \end{minipage}\vspace{0.3em}
&
\begin{minipage}{0.1\textwidth}
    \hbox{\hspace{-0.3em} \includegraphics[width=32mm, height=25.0mm]{./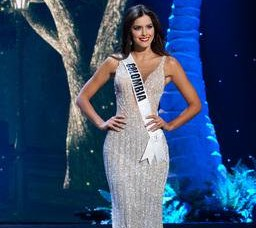}}
  \end{minipage}\vspace{0.3em}
&
\begin{minipage}{0.1\textwidth}
    \hbox{\hspace{-0.3em} \includegraphics[width=34mm, height=25.0mm]{./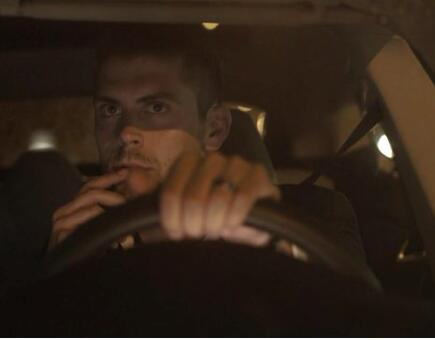}}
  \end{minipage}\vspace{0.3em}
&
\begin{minipage}{0.1\textwidth}
    \hbox{\hspace{-0.3em} \includegraphics[width=34mm, height=25.0mm]{./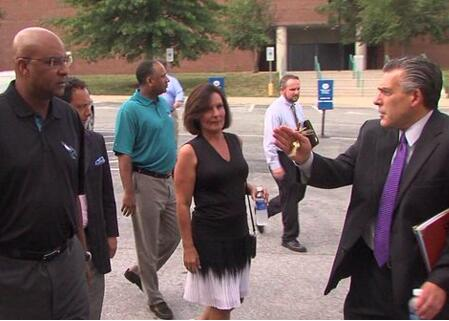}}
  \end{minipage}\vspace{0.3em}\\
\multirow{1}{*}{Text} &
(a) @ WTOP light snow adding to the scenery in \# mclean
&
(b) RT @ TrumpDoral : Congratulations to the the new \# MissUniverse , Miss Colombia , Paulina Vega ! 
& (c) RT @ BleacherReport : VIDEO : Ravens kicker Justin Tucker nails Matthew McConaughey impression in local TV ad
& (d) RT @ myfox8 : Charlotte @ hornets visit \# Greensboro for D - League meeting\\
\midrule
\multirow{3}{*}{GT} &
\multirow{1}{*}{} & (Miss Colombia, POS) & (Ravens, NEU) & (Charlotte, NEU)\\
& (mclean, NEU)& (Paulina Vega, POS)& (Justin Tucker, NEU) & (Greensboro, NEU)\\
& &   & (Matthew McConaughey, NEU) &  (D – League, NEU)\\
\cmidrule{2-5}
\multirow{3}{*}{BART} & 
\multirow{1}{*}{}  & (Colombia, POS)~$\times$ &  (Ravens,  NEU)~$\checkmark$ & (Charlotte, NEU)~$\checkmark$\\
& (WTOP, NEU)~$\times$& (Paulina Vega, POS)~$\checkmark$ & ~~~~~~~~~~~~-~$\times$ & (Greensboro, NEU)~$\checkmark$\\
& &  & (Matthew McConaughey, NEU)~$\checkmark$ & ~~~~~~~~~~~~-~$\times$ \\
\cmidrule{2-5}
\multirow{3}{*}{MM} & 
\multirow{1}{*}{}  & (Colombia, NEU)~$\times$ & (Ravens, NEU)~$\checkmark$ & (Charlotte, NEU)~$\checkmark$\\
& (WTOP, NEU)~$\times$& (Paulina Vega, POS)~$\checkmark$ & (Justin Tucker, POS)$\times$ & (Greensboro, NEU)~$\checkmark$\\
& &  & (Matthew McConaughey, POS)~$\times$ & ~~~~~~~~~~~~-~$\times$ \\
\cmidrule{2-5}
\multirow{3}{*}{Full} & \multirow{1}{*}{}  & (Miss Colombia, POS)~$\checkmark$ & (Ravens, NEU)~$\checkmark$ & (Charlotte, NEU)~$\checkmark$ \\
&(mclean, NEU) ~$\checkmark$ & (Paulina Vega, POS)~$\checkmark$  & (Justin Tucker, NEU)$\checkmark$ & (Greensboro, NEU)~$\checkmark$\\
& &  & (Matthew McConaughey, NEU)~$\checkmark$ & (D – League, NEU)$\checkmark$\\
\bottomrule\\\\
\end{tabular}
\parbox[t]{1\textwidth}{\caption{Predictions of different methods on four test samples. NEU, POS, and NEG respectively denote Neutral, Positive, and Negative sentiments.}\label{tab:appendix}}

% \caption{Predictions of different methods on four test samples. NEU, POS, and NEG respectively denote Neutral, Positive, and Negative sentiments.}
\end{table}

Table.~\ref{tab:appendix} shows four test examples with predictions of different methods. In example (a), both \textit{BART} and \textit{MM} predict the wrong aspect term (e.g., \textit{WTOP}). In example (b), the aspect term \textit{Miss Colombia} is predicted incompletely by \textit{BART} and \textit{MM}. In example (c), \textit{BART} fails to recognize the aspect term \textit{Justin Tucker} while \textit{MM} is able to find it, and this may benefit from the visual information. However, \textit{MM} classifies wrong sentiments towards \textit{Justin Tucker} and \textit{Matthew McConaughey}. In example (d), the two methods without pre-training 
are unable to extract the aspect \textit{D-League}. 
Among all the cases, our \textit{Full} model with pre-training extracts all the aspect terms and classifies corresponding sentiments correctly, which proves the effectiveness of our proposed approach.
